# Supplementary material for: NEO: Saving GPU Memory Crisis with CPU Offloading for Online LLM Inference
Source: arXiv:2411.01142 source file (2024-11-02)
Supplement: Supplementary file 1 [file sec-appendix.tex]

\appendix
\section{Please add supplemental material as appendix here}
Put anything that you might normally include after the references as an appendix here, {\it not in a separate supplementary file}. Upload your final camera-ready as a single pdf, including all appendices.
